# Supplementary material for: A Strong-QCD Regime Measurement of the Proton's Spin Structure
Source: arXiv:2212.00763 source file (2025-05-25)
Supplement: Supplementary file 1 [file thingstoadd.tex]

\chapter{THINGS TO ADD}

Here I want to write even more. Here I want to write even more. Here I want to write even more. Here I want to write even more. Here I want to write even more. Here I want to write even more. Here I want to write even more. Here I want to write even more. Here I want to write even more. Here I want to write even more. Here I want to write even more. Here I want to write even more. Here I want to write even more. Here I want to write even more. Here I want to write even more. Here I want to write even more. Here I want to write even more. Here I want to write even more. Here I want to write even more. Here I want to write even more.
